# Supplementary material for: Towards a General Time Series Anomaly Detector with Adaptive Bottlenecks and Dual Adversarial Decoders
Source: arXiv:2405.15273 source file (2025-03-03)
Supplement: Supplementary file 1 [file appendix-limitations-broader-impacts.tex]

\section{Limitations and broader impacts}\label{sec: limitation}

Time series anomaly detection is important in many application scenarios. Effectively detecting anomalies in time series data helps to identify potential issues in time and takes necessary measures to ensure the normal operation of systems, thereby avoiding possible economic losses and security threats. This is very beneficial to the development of social economy and urban security. Additionally, our model is a general time series anomaly detector with well zero-shot capability, which solves the problem of lack of training data of target scenario due to user privacy, time, labor costs and so on.

One limitation of our model is that we use channel independence for multivariate time series and do not design other special mechanisms for the modeling of the correlation between different time series variables, which may help better anomaly detection in some cases. We would like to leave this as a future work to explore how to capture such correlations under multi-domain pre-training situations. Besides, we mainly use CNNs as the backbone of our model, and we are also willing to explore our model with more other backbones such as RNNs and Transformers.
